# Supplementary material for: Insights on the coupling between vibronically active molecular vibrations and lattice phonons in molecular nanomagnets
Source: arXiv:2106.02611 source file (2021-06-04)
Supplement: Supplementary file 1 [file Dalton_SI.pdf]

# Electronic Supplementary Information for "Insights on the coupling between vibronically active molecular vibrations and lattice phonons in molecular nanomagnets"

Aman Ullah, José J. Baldoví, Alejandro Gaita-Ariño,* and Eugenio Coronado

*Instituto de Ciencia Molecular, Universitat de Valencia, Paterna 46980, Spain*

E-mail: gaita@uv.es

# Supplementary Tables

Table S1: Frequencies ($cm^{-1}$), vibronic coupling ($S_n$ ($cm^{-1}$) at CASSCF level for optimized geometry for each normal mode ($n$) and vibronic-phonon couplings $S(\mu_{n,xx})$, $S(\mu_{n,xy})$, $S(\mu_{n,xz})$.

| Modes (n) | Frequencies ($cm^{-1}$) | $S_n$ ($cm^{-1}$) | S (n, $\mu_{xx}$) | S (n, $\mu_{xy}$) | S (n, $\mu_{xz}$) |
|---|---|---|---|---|---|
| 1 | 8.62 | 0.085 | 0.01 | 0.01 | 0.01 |
| 2 | 17.94 | 0.176 | 0.14 | 0.03 | 0.01 |
| 3 | 18.43 | 0.119 | 0.03 | 0.04 | 0.01 |
| 4 | 24.33 | 0.247 | 0.00 | 0.13 | 0.01 |
| 5 | 29.97 | 0.220 | 0.01 | 0.01 | 0.13 |
| 6 | 43.22 | 0.123 | 0.91 | 0.01 | 0.01 |
| 7 | 54.02 | 0.150 | 0.26 | 0.03 | 0.00 |
| 8 | 58.39 | 0.180 | 0.01 | 0.01 | 0.03 |
| 9 | 67.12 | 0.145 | 0.17 | 0.01 | 0.00 |
| 10 | 70.95 | 0.130 | 0.04 | 0.05 | 0.01 |
| 11 | 99.61 | 0.125 | 0.01 | 0.07 | 0.01 |
| 12 | 106.52 | 0.151 | 0.02 | 0.01 | 0.07 |
| 13 | 106.78 | 0.051 | 0.01 | 0.01 | 0.04 |
| 14 | 107.26 | 0.132 | 0.00 | 0.06 | 0.01 |
| 15 | 108.76 | 0.167 | 0.01 | 0.00 | 0.00 |
| 16 | 114.68 | 0.067 | 0.01 | 0.00 | 0.00 |
| 17 | 114.71 | 0.080 | 0.01 | 0.00 | 0.00 |
| 18 | 140.11 | 0.109 | 0.01 | 0.01 | 0.00 |
| 19 | 140.76 | 0.040 | 0.04 | 0.00 | 0.01 |
| 20 | 141.19 | 0.038 | 0.00 | 0.01 | 0.04 |
| 21 | 142.11 | 0.129 | 0.01 | 0.04 | 0.00 |

Table S1: Continued from previous page

| Modes (n) | Frequencies ($cm^{-1}$) | $S_n$ ($cm^{-1}$) | S (n, $\mu_{xx}$) | S (n, $\mu_{xy}$) | S (n, $\mu_{xz}$) |
|---|---|---|---|---|---|
| 22 | 143.98 | 0.123 | 0.09 | 0.01 | 0.00 |
| 23 | 144.75 | 0.039 | 0.02 | 0.06 | 0.00 |
| 24 | 157.60 | 0.020 | 0.00 | 0.00 | 0.02 |
| 25 | 158.17 | 0.081 | 0.00 | 0.02 | 0.23 |
| 26 | 159.14 | 0.096 | 0.00 | 0.28 | 0.02 |
| 27 | 159.88 | 0.042 | 0.00 | 0.08 | 0.03 |
| 28 | 160.56 | 0.039 | 0.00 | 0.03 | 0.12 |
| 29 | 161.30 | 0.079 | 0.01 | 0.06 | 0.08 |
| 30 | 167.76 | 0.094 | 0.00 | 0.00 | 0.00 |
| 31 | 167.77 | 0.083 | 0.01 | 0.02 | 0.00 |
| 32 | 184.62 | 0.122 | 0.00 | 0.00 | 0.01 |
| 33 | 184.73 | 0.122 | 0.00 | 0.01 | 0.00 |
| 34 | 193.02 | 0.038 | 0.01 | 0.01 | 0.01 |
| 35 | 202.14 | 0.095 | 0.15 | 0.00 | 0.00 |
| 36 | 216.40 | 0.027 | 0.02 | 0.02 | 0.01 |
| 37 | 216.89 | 0.066 | 0.00 | 0.02 | 0.03 |
| 38 | 218.12 | 0.088 | 0.00 | 0.00 | 0.06 |
| 39 | 218.13 | 0.099 | 0.01 | 0.02 | 0.06 |
| 40 | 218.22 | 0.126 | 0.01 | 0.11 | 0.08 |
| 41 | 218.24 | 0.117 | 0.00 | 0.11 | 0.07 |
| 42 | 219.96 | 0.057 | 0.01 | 0.01 | 0.02 |
| 43 | 220.00 | 0.054 | 0.00 | 0.14 | 0.02 |
| 44 | 220.07 | 0.115 | 0.00 | 0.01 | 0.18 |
| 45 | 220.47 | 0.111 | 0.03 | 0.05 | 0.02 |

Table S1: Continued from previous page

| Modes (n) | Frequencies ($cm^{-1}$) | $S_n$ ($cm^{-1}$) | S (n, $\mu_{xx}$) | S (n, $\mu_{xy}$) | S (n, $\mu_{xz}$) |
|---|---|---|---|---|---|
| 46 | 223.18 | 0.079 | 0.05 | 0.08 | 0.01 |
| 47 | 224.41 | 0.072 | 0.05 | 0.04 | 0.01 |
| 48 | 230.85 | 0.034 | 0.01 | 0.01 | 0.00 |
| 49 | 231.24 | 0.031 | 0.01 | 0.01 | 0.02 |
| 50 | 231.75 | 0.036 | 0.00 | 0.02 | 0.02 |
| 51 | 232.10 | 0.036 | 0.01 | 0.02 | 0.00 |
| 52 | 235.13 | 0.019 | 0.00 | 0.00 | 0.01 |
| 53 | 235.33 | 0.029 | 0.01 | 0.00 | 0.00 |
| 54 | 257.49 | 0.097 | 0.00 | 0.00 | 0.00 |
| 55 | 257.49 | 0.108 | 0.01 | 0.00 | 0.00 |
| 56 | 289.55 | 0.030 | 0.00 | 0.00 | 0.00 |
| 57 | 291.07 | 0.025 | 0.00 | 0.00 | 0.00 |
| 58 | 329.19 | 0.091 | 0.00 | 0.00 | 0.02 |
| 59 | 329.25 | 0.125 | 0.00 | 0.02 | 0.01 |
| 60 | 337.26 | 0.101 | 0.00 | 0.02 | 0.02 |
| 61 | 337.36 | 0.143 | 0.00 | 0.02 | 0.04 |
| 62 | 337.40 | 0.099 | 0.00 | 0.03 | 0.00 |
| 63 | 337.72 | 0.101 | 0.00 | 0.02 | 0.01 |
| 64 | 351.19 | 0.101 | 0.00 | 0.08 | 0.03 |
| 65 | 354.95 | 0.147 | 0.00 | 0.07 | 0.21 |
| 66 | 355.21 | 0.148 | 0.00 | 0.20 | 0.08 |
| 67 | 359.02 | 0.064 | 0.01 | 0.00 | 0.00 |
| 68 | 360.26 | 0.032 | 0.02 | 0.01 | 0.00 |
| 69 | 363.49 | 0.085 | 0.00 | 0.04 | 0.02 |

Table S1: Continued from previous page

| Modes (n) | Frequencies (cm$^{-1}$) | S$_n$ (cm$^{-1}$) | S (n, $\mu_{xx}$) | S (n, $\mu_{xy}$) | S (n, $\mu_{xz}$) |
|---|---|---|---|---|---|
| 70 | 399.03 | 0.041 | 0.02 | 0.05 | 0.06 |
| 71 | 399.78 | 0.067 | 0.01 | 0.07 | 0.05 |
| 72 | 399.80 | 0.053 | 0.02 | 0.01 | 0.03 |
| 73 | 404.19 | 0.083 | 0.30 | 0.00 | 0.00 |
| 74 | 414.55 | 0.141 | 0.01 | 0.26 | 0.03 |
| 75 | 414.92 | 0.126 | 0.00 | 0.04 | 0.27 |
| 76 | 416.67 | 0.116 | 0.00 | 0.07 | 0.18 |
| 77 | 416.90 | 0.111 | 0.04 | 0.14 | 0.06 |
| 78 | 417.53 | 0.131 | 0.02 | 0.10 | 0.06 |
| 79 | 417.69 | 0.120 | 0.02 | 0.06 | 0.04 |
| 80 | 429.95 | 0.091 | 0.00 | 0.03 | 0.00 |
| 81 | 431.15 | 0.065 | 0.35 | 0.01 | 0.00 |
| 82 | 435.19 | 0.083 | 0.01 | 0.01 | 0.17 |
| 83 | 436.31 | 0.046 | 0.03 | 0.05 | 0.05 |
| 84 | 436.72 | 0.078 | 0.07 | 0.15 | 0.03 |
| 85 | 437.91 | 0.056 | 0.15 | 0.08 | 0.00 |
| 86 | 479.05 | 0.084 | 0.00 | 0.21 | 0.01 |
| 87 | 479.34 | 0.070 | 0.00 | 0.01 | 0.21 |
| 88 | 480.96 | 0.037 | 0.01 | 0.01 | 0.00 |
| 89 | 481.29 | 0.038 | 0.00 | 0.00 | 0.03 |
| 90 | 489.34 | 0.055 | 0.00 | 0.02 | 0.01 |
| 91 | 489.38 | 0.054 | 0.00 | 0.00 | 0.02 |
| 92 | 514.29 | 0.028 | 0.00 | 0.00 | 0.00 |
| 93 | 515.09 | 0.031 | 0.01 | 0.00 | 0.01 |

Table S1: Continued from previous page

| Modes (n) | Frequencies (cm$^{-1}$) | S$_n$ (cm$^{-1}$) | S (n, $\mu_{xx}$) | S (n, $\mu_{xy}$) | S (n, $\mu_{xz}$) |
|---|---|---|---|---|---|
| 94 | 515.25 | 0.029 | 0.02 | 0.00 | 0.01 |
| 95 | 516.21 | 0.076 | 0.12 | 0.00 | 0.00 |
| 96 | 520.31 | 0.113 | 0.00 | 0.01 | 0.01 |
| 97 | 521.09 | 0.102 | 0.01 | 0.01 | 0.01 |
| 98 | 528.07 | 0.086 | 0.04 | 0.01 | 0.00 |
| 99 | 529.22 | 0.079 | 0.01 | 0.00 | 0.01 |
| 100 | 530.46 | 0.069 | 0.09 | 0.00 | 0.00 |
| 101 | 531.81 | 0.080 | 0.19 | 0.01 | 0.00 |
| 102 | 535.59 | 0.091 | 0.00 | 0.00 | 0.01 |
| 103 | 536.21 | 0.097 | 0.05 | 0.02 | 0.00 |
| 104 | 554.98 | 0.020 | 0.00 | 0.00 | 0.00 |
| 105 | 555.04 | 0.018 | 0.00 | 0.00 | 0.00 |
| 106 | 578.43 | 0.031 | 0.01 | 0.14 | 0.01 |
| 107 | 579.04 | 0.042 | 0.01 | 0.06 | 0.11 |
| 108 | 579.13 | 0.027 | 0.02 | 0.14 | 0.01 |
| 109 | 579.49 | 0.033 | 0.00 | 0.02 | 0.18 |
| 110 | 671.58 | 0.235 | 0.00 | 0.25 | 0.01 |

Table S2: For normal mode n, vibronic-phonon couplings $S(\mu_{n,yx})$, $S(\mu_{n,yy})$, $S(\mu_{n,yz})$, $S(\mu_{n,zx})$, $S(\mu_{n,zy})$, $S(\mu_{n,zz})$.

| Modes (n) | S (n, $\mu_{yx}$) | S (n, $\mu_{yy}$) | S (n, $\mu_{yz}$) | S (n, $\mu_{zx}$) | S (n, $\mu_{zy}$) | S (n, $\mu_{zz}$) |
|---|---|---|---|---|---|---|
| 1 | 0.03 | 0.01 | 0.00 | 0.04 | 0.00 | 0.00 |
| 2 | 0.13 | 0.03 | 0.00 | 0.02 | 0.01 | 0.04 |
| 3 | 0.21 | 0.01 | 0.02 | 0.04 | 0.02 | 0.01 |

Table S2: Continued from previous page

| Modes (n) | S (n, $\mu_{yx}$) | S (n, $\mu_{yy}$) | S (n, $\mu_{yz}$) | S (n, $\mu_{zx}$) | S (n, $\mu_{zy}$) | S (n, $\mu_{zz}$) |
|---|---|---|---|---|---|---|
| 4 | 0.65 | 0.05 | 0.01 | 0.05 | 0.01 | 0.05 |
| 5 | 0.06 | 0.01 | 0.04 | 0.69 | 0.05 | 0.01 |
| 6 | 0.06 | 0.00 | 0.01 | 0.00 | 0.00 | 0.06 |
| 7 | 0.14 | 0.31 | 0.02 | 0.01 | 0.02 | 0.25 |
| 8 | 0.02 | 0.03 | 0.33 | 0.11 | 0.34 | 0.02 |
| 9 | 0.05 | 0.20 | 0.01 | 0.01 | 0.01 | 0.28 |
| 10 | 0.03 | 0.03 | 0.07 | 0.01 | 0.08 | 0.03 |
| 11 | 0.32 | 0.00 | 0.01 | 0.04 | 0.01 | 0.00 |
| 12 | 0.04 | 0.01 | 0.01 | 0.41 | 0.01 | 0.01 |
| 13 | 0.06 | 0.01 | 0.01 | 0.27 | 0.01 | 0.01 |
| 14 | 0.43 | 0.00 | 0.00 | 0.05 | 0.02 | 0.00 |
| 15 | 0.08 | 0.07 | 0.06 | 0.01 | 0.08 | 0.07 |
| 16 | 0.03 | 0.13 | 0.15 | 0.00 | 0.14 | 0.13 |
| 17 | 0.01 | 0.10 | 0.10 | 0.03 | 0.08 | 0.08 |
| 18 | 0.12 | 0.02 | 0.02 | 0.00 | 0.02 | 0.02 |
| 19 | 0.01 | 0.12 | 0.01 | 0.00 | 0.00 | 0.14 |
| 20 | 0.01 | 0.00 | 0.01 | 0.18 | 0.00 | 0.00 |
| 21 | 0.17 | 0.05 | 0.04 | 0.02 | 0.01 | 0.06 |
| 22 | 0.03 | 0.38 | 0.00 | 0.00 | 0.01 | 0.37 |
| 23 | 0.02 | 0.05 | 0.08 | 0.04 | 0.01 | 0.03 |
| 24 | 0.01 | 0.00 | 0.45 | 0.02 | 0.45 | 0.01 |
| 25 | 0.02 | 0.00 | 0.03 | 0.20 | 0.04 | 0.01 |
| 26 | 0.23 | 0.01 | 0.06 | 0.01 | 0.04 | 0.01 |
| 27 | 0.06 | 0.05 | 0.14 | 0.02 | 0.11 | 0.03 |
| 28 | 0.02 | 0.01 | 0.17 | 0.09 | 0.18 | 0.00 |

Table S2: Continued from previous page

| Modes (n) | S (n, $\mu_{yx}$) | S (n, $\mu_{yy}$) | S (n, $\mu_{yz}$) | S (n, $\mu_{zx}$) | S (n, $\mu_{zy}$) | S (n, $\mu_{zz}$) |
|---|---|---|---|---|---|---|
| 29 | 0.03 | 0.03 | 0.15 | 0.07 | 0.21 | 0.01 |
| 30 | 0.01 | 0.35 | 0.19 | 0.01 | 0.19 | 0.35 |
| 31 | 0.02 | 0.19 | 0.38 | 0.01 | 0.33 | 0.19 |
| 32 | 0.00 | 0.00 | 0.01 | 0.01 | 0.01 | 0.00 |
| 33 | 0.01 | 0.03 | 0.01 | 0.00 | 0.00 | 0.01 |
| 34 | 0.02 | 0.01 | 0.00 | 0.00 | 0.00 | 0.01 |
| 35 | 0.00 | 0.17 | 0.02 | 0.00 | 0.01 | 0.19 |
| 36 | 0.01 | 0.04 | 0.02 | 0.00 | 0.01 | 0.06 |
| 37 | 0.03 | 0.01 | 0.09 | 0.01 | 0.08 | 0.04 |
| 38 | 0.00 | 0.15 | 0.17 | 0.03 | 0.16 | 0.16 |
| 39 | 0.00 | 0.18 | 0.12 | 0.03 | 0.12 | 0.17 |
| 40 | 0.04 | 0.04 | 0.05 | 0.03 | 0.05 | 0.05 |
| 41 | 0.06 | 0.06 | 0.09 | 0.02 | 0.09 | 0.03 |
| 42 | 0.02 | 0.05 | 0.01 | 0.02 | 0.01 | 0.01 |
| 43 | 0.16 | 0.02 | 0.01 | 0.02 | 0.01 | 0.03 |
| 44 | 0.01 | 0.01 | 0.02 | 0.20 | 0.02 | 0.00 |
| 45 | 0.06 | 0.10 | 0.03 | 0.01 | 0.05 | 0.06 |
| 46 | 0.09 | 0.10 | 0.01 | 0.01 | 0.02 | 0.09 |
| 47 | 0.07 | 0.07 | 0.02 | 0.01 | 0.04 | 0.10 |
| 48 | 0.00 | 0.01 | 0.01 | 0.01 | 0.00 | 0.00 |
| 49 | 0.00 | 0.00 | 0.00 | 0.02 | 0.00 | 0.01 |
| 50 | 0.00 | 0.01 | 0.00 | 0.02 | 0.02 | 0.01 |
| 51 | 0.04 | 0.00 | 0.01 | 0.00 | 0.01 | 0.01 |
| 52 | 0.00 | 0.00 | 0.18 | 0.00 | 0.18 | 0.00 |
| 53 | 0.01 | 0.00 | 0.11 | 0.00 | 0.11 | 0.00 |

Table S2: Continued from previous page

| Modes (n) | S (n, $\mu_{yx}$) | S (n, $\mu_{yy}$) | S (n, $\mu_{yz}$) | S (n, $\mu_{zx}$) | S (n, $\mu_{zy}$) | S (n, $\mu_{zz}$) |
|---|---|---|---|---|---|---|
| 54 | 0.00 | 0.01 | 0.00 | 0.00 | 0.01 | 0.01 |
| 55 | 0.02 | 0.00 | 0.01 | 0.01 | 0.01 | 0.00 |
| 56 | 0.00 | 0.00 | 0.02 | 0.00 | 0.01 | 0.00 |
| 57 | 0.01 | 0.00 | 0.00 | 0.00 | 0.00 | 0.00 |
| 58 | 0.00 | 0.01 | 0.10 | 0.02 | 0.10 | 0.01 |
| 59 | 0.03 | 0.10 | 0.01 | 0.01 | 0.02 | 0.10 |
| 60 | 0.03 | 0.01 | 0.01 | 0.03 | 0.00 | 0.00 |
| 61 | 0.02 | 0.00 | 0.00 | 0.05 | 0.00 | 0.00 |
| 62 | 0.05 | 0.00 | 0.00 | 0.01 | 0.00 | 0.00 |
| 63 | 0.01 | 0.00 | 0.01 | 0.04 | 0.01 | 0.01 |
| 64 | 0.14 | 0.01 | 0.00 | 0.06 | 0.00 | 0.00 |
| 65 | 0.12 | 0.00 | 0.01 | 0.39 | 0.01 | 0.00 |
| 66 | 0.37 | 0.00 | 0.01 | 0.15 | 0.00 | 0.00 |
| 67 | 0.01 | 0.05 | 0.00 | 0.00 | 0.01 | 0.05 |
| 68 | 0.02 | 0.05 | 0.00 | 0.01 | 0.00 | 0.06 |
| 69 | 0.08 | 0.02 | 0.01 | 0.04 | 0.02 | 0.02 |
| 70 | 0.02 | 0.02 | 0.04 | 0.02 | 0.03 | 0.03 |
| 71 | 0.03 | 0.02 | 0.02 | 0.02 | 0.02 | 0.03 |
| 72 | 0.00 | 0.01 | 0.01 | 0.00 | 0.00 | 0.03 |
| 73 | 0.00 | 0.12 | 0.00 | 0.00 | 0.00 | 0.11 |
| 74 | 0.02 | 0.10 | 0.00 | 0.00 | 0.00 | 0.09 |
| 75 | 0.00 | 0.01 | 0.09 | 0.01 | 0.09 | 0.01 |
| 76 | 0.00 | 0.02 | 0.06 | 0.00 | 0.06 | 0.01 |
| 77 | 0.01 | 0.00 | 0.03 | 0.01 | 0.03 | 0.01 |
| 78 | 0.01 | 0.16 | 0.05 | 0.01 | 0.05 | 0.17 |

Table S2: Continued from previous page

| Modes (n) | S (n, $\mu_{yx}$) | S (n, $\mu_{yy}$) | S (n, $\mu_{yz}$) | S (n, $\mu_{zx}$) | S (n, $\mu_{zy}$) | S (n, $\mu_{zz}$) |
|---|---|---|---|---|---|---|
| 79 | 0.02 | 0.05 | 0.16 | 0.01 | 0.16 | 0.05 |
| 80 | 0.12 | 0.01 | 0.00 | 0.00 | 0.01 | 0.01 |
| 81 | 0.01 | 0.05 | 0.01 | 0.00 | 0.01 | 0.06 |
| 82 | 0.01 | 0.00 | 0.01 | 0.31 | 0.02 | 0.00 |
| 83 | 0.09 | 0.01 | 0.01 | 0.07 | 0.01 | 0.00 |
| 84 | 0.25 | 0.02 | 0.01 | 0.04 | 0.01 | 0.00 |
| 85 | 0.12 | 0.01 | 0.00 | 0.01 | 0.00 | 0.03 |
| 86 | 0.06 | 0.01 | 0.00 | 0.00 | 0.00 | 0.01 |
| 87 | 0.00 | 0.00 | 0.01 | 0.05 | 0.01 | 0.00 |
| 88 | 0.01 | 0.01 | 0.00 | 0.00 | 0.00 | 0.02 |
| 89 | 0.00 | 0.00 | 0.01 | 0.00 | 0.01 | 0.00 |
| 90 | 0.01 | 0.06 | 0.00 | 0.00 | 0.00 | 0.06 |
| 91 | 0.00 | 0.00 | 0.06 | 0.01 | 0.06 | 0.00 |
| 92 | 0.00 | 0.00 | 0.01 | 0.00 | 0.01 | 0.01 |
| 93 | 0.00 | 0.02 | 0.04 | 0.00 | 0.05 | 0.02 |
| 94 | 0.00 | 0.04 | 0.02 | 0.01 | 0.03 | 0.04 |
| 95 | 0.00 | 0.24 | 0.00 | 0.00 | 0.01 | 0.23 |
| 96 | 0.02 | 0.04 | 0.04 | 0.01 | 0.03 | 0.04 |
| 97 | 0.01 | 0.03 | 0.04 | 0.01 | 0.04 | 0.05 |
| 98 | 0.01 | 0.04 | 0.00 | 0.00 | 0.00 | 0.04 |
| 99 | 0.00 | 0.01 | 0.00 | 0.01 | 0.00 | 0.01 |
| 100 | 0.01 | 0.06 | 0.00 | 0.00 | 0.00 | 0.08 |
| 101 | 0.00 | 0.13 | 0.00 | 0.00 | 0.00 | 0.14 |
| 102 | 0.00 | 0.00 | 0.05 | 0.00 | 0.05 | 0.01 |
| 103 | 0.00 | 0.08 | 0.01 | 0.00 | 0.00 | 0.02 |

Table S2: Continued from previous page

| Modes (n) | S (n, $\mu_{yx}$) | S (n, $\mu_{yy}$) | S (n, $\mu_{yz}$) | S (n, $\mu_{zx}$) | S (n, $\mu_{zy}$) | S (n, $\mu_{zz}$) |
|---|---|---|---|---|---|---|
| 104 | 0.00 | 0.25 | 0.01 | 0.00 | 0.01 | 0.25 |
| 105 | 0.00 | 0.00 | 0.25 | 0.00 | 0.25 | 0.01 |
| 106 | 0.10 | 0.00 | 0.00 | 0.01 | 0.00 | 0.00 |
| 107 | 0.05 | 0.00 | 0.01 | 0.08 | 0.01 | 0.01 |
| 108 | 0.09 | 0.01 | 0.00 | 0.01 | 0.00 | 0.01 |
| 109 | 0.01 | 0.00 | 0.01 | 0.13 | 0.01 | 0.00 |
| 110 | 0.20 | 0.02 | 0.01 | 0.01 | 0.00 | 0.02 |
